# Supplementary material for: The Emergence of Reproducibility and Generalizability in Diffusion Models
Source: arXiv:2310.05264 source file (2026-06-09)
Supplement: Supplementary file 1 [file Appendix_othergm.tex]

\section{Compare GAN \& VAE}
\label{append:compare_other_gm}

% \begin{\figure}[t]{0.5\textwidth}
%     \centering
%     \includegraphics[width=1.0\linewidth]{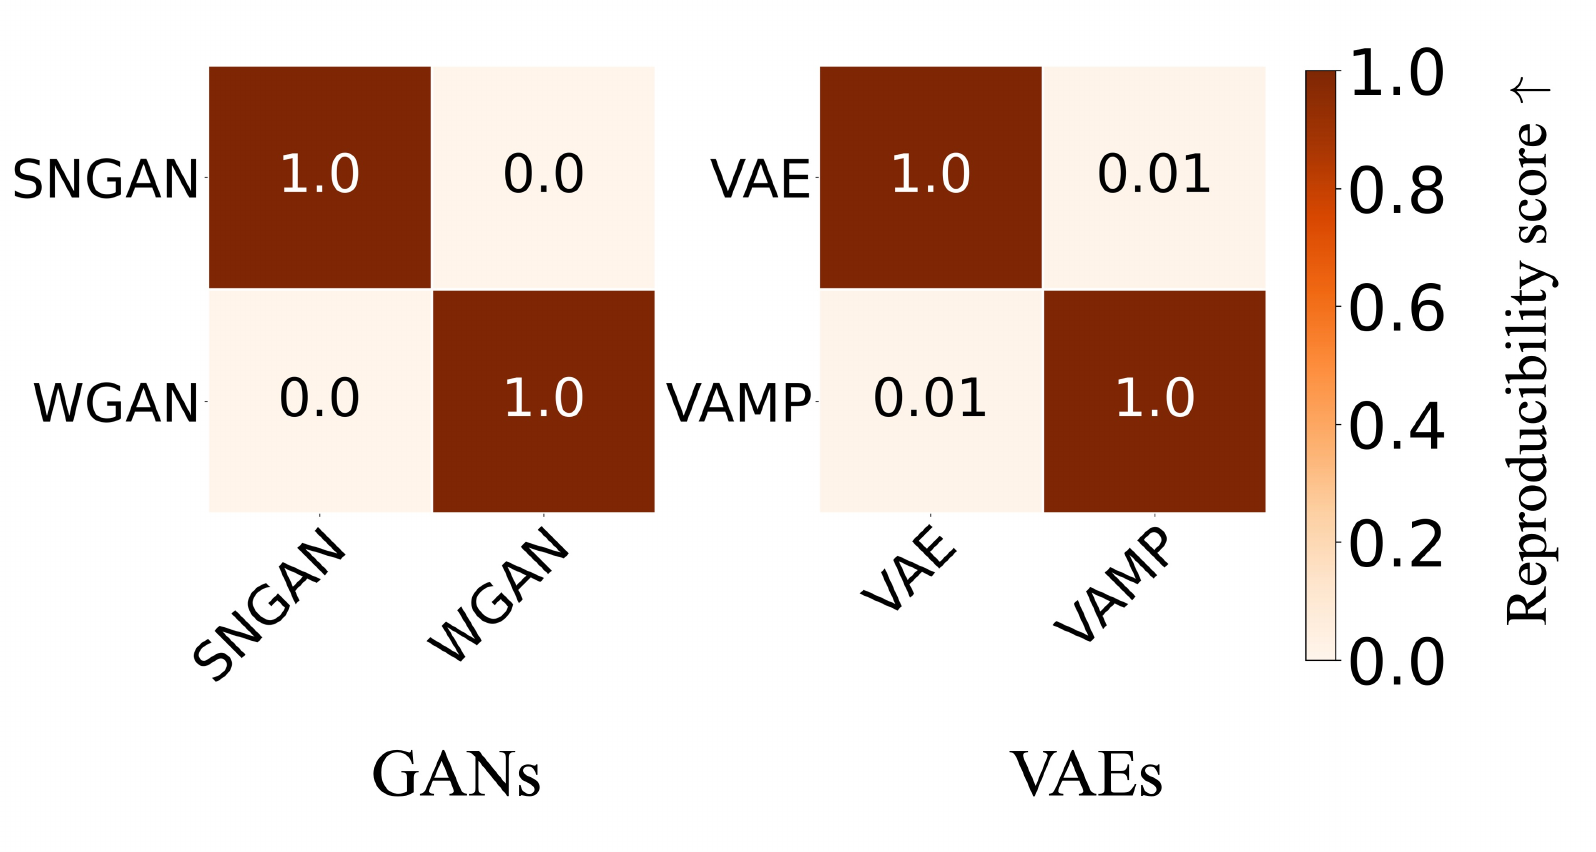}
%          % \caption{Reproducibilty between theoretical and experiment results}
%     \caption{Quantitative results for GANS and VAEs.}
%     \label{fig:gan_and_vae}
% \end{\figure}

\begin{figure}[t]
    \centering
    \includegraphics[width=0.5\linewidth]{figure/gan_vae/gan_nad_vae_v4.pdf}
    \caption{\textbf{Quantitative results for GANS and VAEs.}}
    \label{fig:gan_and_vae}
\end{figure}

% As a comparison of this observation in the diffusion model, we assess model similarity for both Generative Adversarial Network (GAN) \cite{goodfellow2014generative} and Variational Autoencoder (VAE) \cite{kingma2013auto} based approaches using the reproducibility score. In our evaluation, for GAN-based methods, we contrast wGAN \cite{arjovsky2017wasserstein} and SNGAN \cite{miyato2018spectral} using CIFAR-10. Meanwhile, for VAE-based approaches, we consider both VAE and VAMP \cite{tomczak2018vae} on MNIST dataset \cite{deng2012mnist}. All models are released by the author and the reproducibility score is calculated similarly to the diffusion model. Note that the latent space of the VAE-based method is learned from the encoder, which is different for different models. Here, we sample initial noise from the latent space of one model and use it for the generation of the other. 

% The similarity matrices presented in \Cref{fig:gan_and_vae} imply a lack of reproducibility in both GAN and VAE methods.

To further investigate this observation within the realm of diffusion models, we extend our assessment to model similarity in Generative Adversarial Networks (GANs) \cite{goodfellow2014generative} and Variational Autoencoders (VAEs) \cite{kingma2013auto}. We gauge this similarity through the application of a reproducibility score. In our evaluation of GAN-based methods, we contrast two prominent variants: Wasserstein GAN (wGAN) \cite{arjovsky2017wasserstein} and Spectral Normalization GAN (SNGAN) \cite{miyato2018spectral}. We conduct this analysis using the CIFAR-10 dataset. Simultaneously, within the realm of VAE-based approaches, we consider both the standard VAE and the Variational Autoencoding Mutual Information Bottleneck (VAMP) model \cite{tomczak2018vae}. Our evaluation focuses on the MNIST dataset introduced by Deng \cite{lecun1998gradient}. It's important to note that each model utilized in this analysis was provided by its respective author, and the reproducibility score calculation follows a similar methodology to that applied in the diffusion model experiments. Of particular significance is the fact that the latent space for VAE-based methods is learned through the encoder, and this encoder architecture varies among different models. In this context, our approach involves sampling initial noise from the latent space of one model and employing it for the generation of another. The similarity matrices, presented in \Cref{fig:gan_and_vae}, collectively indicate a notable absence of reproducibility in both GAN and VAE methods.
