# Supplementary material for: The Emergence of Reproducibility and Generalizability in Diffusion Models
Source: arXiv:2310.05264 source file (2026-06-09)
Supplement: Supplementary file 5 [file Appendix_summary.tex]

% \par\noindent\rule{\textwidth}{1pt}
% \begin{center}
% {\Large \bf Appendix}
% \end{center}
% \vspace{-0.1in}
% \par\noindent\rule{\textwidth}{1pt}

% \vspace{0.2in}

% \startcontents[sections]
% \printcontents[sections]{l}{1}{\setcounter{tocdepth}{2}}

% \vspace{0.2in}

% We include more comprehensive experiment settings, quantitative results, and detailed discussion of the unconditional diffusion model in \Cref{append:unconditional}, theoretical analysis on "memorization regime"  in \Cref{append:theory}, conditional diffusion model in \Cref{append:conditional}, diffusion model for solving inverse problems in \Cref{append:inverseproblem}, fine-tuning diffusion model in \Cref{append:fintuning}. Quantitative analysis of other generative models is in \Cref{append:compare_other_gm}. Proof for \Cref{theorem:unique_identitical_encoding} could also be found in \Cref{append:theory}.
